# Supplementary material for: Setting the Right Expectations: Algorithmic Recourse Over Time
Source: arXiv:2309.06969 source file (2023-09-13)
Supplement: Supplementary file 1 [file appendix.tex]

\appendix
 
\section{Understanding the Effects of Different Parameters}

The proposed framework allows a policy-maker to understand the impact of a given setting where algorithmic recourse might be introduced. An example of this analysis is shown in Figure \ref{fig:rate-positive-outcomes-comparison}. This figure focuses on the more competitive scenarios, where 12 new agents are introduced every time-step. In such settings, the discrepancy between applied effort and expected reward becomes clear; Sub groups with a lower initial score have a much lower expectation of receiving a favorable outcome, when compared to sub groups with higher initial score, with a similar or superior effort, even with similar rates of adaptation (as is the case of the approach \hl{using continuous adaptation with constant effort}).

\begin{figure}
    \centering
    \includegraphics[width=1.0\linewidth]{figures/rate_positive_outcomes_comparison.pdf}
    \caption{Analysis of the number of favorable outcomes as a percentage of the groups' size. Groups are formed based on their initial score, where the group named ``Lowest''/``Highest'' represents the sub-population with the lowest/highest initial scores. Rates are averaged over 20 random seeds. Every scenario presented introduces 12 new agents per time-step.}
    \label{fig:rate-positive-outcomes-comparison}
\end{figure}

The inequality effect described above can also be observed, to a lower extent, in Figure \ref{fig:single-run-adaptive-scores-panel}. It shows the simulations described in our experimental results, over a single run. In this case, it is possible to observe the trails of agents' adaptations across time-steps. In scenarios where the threshold tends to increase, agents with a lower initial score end up having to reach higher scores the longer they remain in the environment. Eventually, the effort required for agents with a lower initial score becomes disproportionately higher than the one required by agents with a higher initial score.

\begin{figure}
    \centering
    \includegraphics[width=1.0\linewidth]{figures/single_run_gaussian_adaptation_scores_panel.jpeg}
    \caption{Threshold values and agents' scores along 50 time-steps for a single run. \hl{Continuous adaptation with flexible effort approach}, updated every time-step (global adaptation is determined along the y-axis). Number of new agents per time-step is determined along the x-axis.}
    \label{fig:single-run-adaptive-scores-panel}
\end{figure}

This effect may also be reflected in the recourse reliability score $RR_t$ presented in Figure \ref{fig:single-run-adaptive-success-panel}. This figure shows the existence of two challenges that must be taken into consideration: (1) over time, the trend of the recourse reliability $RR_t$ and threshold $y_t$ decay should be simultaneously stable, and (2) the volatility of the recourse reliability $RR_t$ should be reduced whenever possible. These challenges become more important as the competitiveness level of the environment increases (\textit{i.e.}, the higher number of new agents and/or the global rate of adaptation).

\begin{figure}
    \centering
    \includegraphics[width=1.0\linewidth]{figures/single_run_gaussian_adaptation_success_panel.pdf}
    \caption{Recourse Reliability score $RR_t$ along 50 time-steps for a single run. \hl{Continuous adaptation with flexible effort approach}, updated every time-step (global adaptation is determined along the y-axis). Number of new agents per time-step is determined along the x-axis.}
    \label{fig:single-run-adaptive-success-panel}
\end{figure}

\section{Understanding the Population's Behavior}~\label{ap:population-behavior}

We may also look into the behavior of a single population and analyze how different agents behave and progress comparatively to the remaining agents. To do this, we will focus on a specific environment, within the ones presented in Figure \ref{fig:single-run-adaptive-scores-panel}, using the \hl{continuous adaptation with flexible effort approach}, with 10 new agents per time-step and a global adaptation rate of 0.3.
Figure \ref{fig:agents_scores_distribution} shows the progression of the population's score distribution over three different time-steps. Over the different time-steps, the scores' distribution tends to shift to the right, towards higher scores. This may be considered as an improvement of the population's social welfare. Intuitively, settings with higher adaptation rates will tend to skew this distribution further to the right, and reduce its variability. However, as the recourse reliability lowers (along with the agents' individual welfare), the social welfare improves, and the trade off previously discussed becomes clearer. This particular setting shows it may be possible to strike a balance among the two, since the recourse reliability remains relatively high (although with high variability), the population's score distribution is shifting upwards, while the threshold also increases.

\begin{figure}[H]
    \centering
    \includegraphics[width=1.0\linewidth]{figures/agents_scores_distribution_adaptation_0.3_new_agents_10.pdf}
    \caption{Agent scores' distribution. \hl{Approach: continuous adaptation with flexible effort}, Adaptation rate: 0.3, New agents: 10.}
    \label{fig:agents_scores_distribution}
\end{figure}

Any particular time-step may also be analysed at a lower level. Specifically, Figure \ref{fig:agents_scatter_plot} shows how the population behaved at $t=5$. In this particular time-step, the threshold increased, compared to $t=4$, since several agents adapted to reach a score above the previous threshold. This led to a some agents surpassing the previous threshold and still failing to receive a favorable outcome, since there were at least 10 other agents that achieved a higher score. In this figure the effect of the adaptation function over the entire population is also visible. Since the \hl{continuous adaptation with flexible effort} approach conditions an agent to adapt based on its distance to the threshold, the observations closer to the threshold are adapting to a higher degree than the ones further away from away it.

\begin{figure}
    \centering
    \includegraphics[width=1.0\linewidth]{figures/agents_scatter_plot_adaptation_0.3_new_agents_10.pdf}
    \caption{Agents adapting towards the the target threshold. \hl{Approach: continuous adaptation with flexible effort}, time-step: 5, Adaptation rate: 0.3, New agents: 10.}
    \label{fig:agents_scatter_plot}
\end{figure}
